# Supplementary material for: Leroy and Blazy were right: their memory model soundness proof is automatable (Extended Version)
Source: arXiv:2212.02425 source file (2022-12-05)
Supplement: Supplementary file 1 [file appendix2.tex]

\section{Proof statistics of modules GEN\_MEM and REF\_GEN\_MEM}
%GEN_MEM
\begin{table}[ht]
\begin{minipage}{.5\linewidth}
      
    \centering
        \scalebox{0.8}{
        
        \begin{tabular}{|l|c|}
        \hline \multicolumn{1}{|c|}{Proof obligations } & \provername{Alt-Ergo 2.4.1} \\ 
        \hline
        \explanation{alloc\_valid\_block\_inv} & \valid{0.00} \\ 
        \hline
        \explanation{alloc\_not\_valid\_block\_2} & \valid{0.00} \\ 
        \hline
        \explanation{load\_alloc\_other\_2} & \valid{0.00} \\ 
        \hline
        \explanation{alloc\_result\_valid\_pointer} & \valid{0.01} \\ 
        \hline
        \explanation{alloc\_valid\_pointer\_inv} & \valid{0.01} \\ 
        \hline
        \explanation{store\_valid\_pointer\_inv} & \valid{0.01} \\ 
        \hline
        \explanation{free\_valid\_pointer\_inv} & \valid{0.01} \\ 
        \hline 
        
        \end{tabular}

        }
    \medskip
    \caption{Proof stats of GEN\_MEM}
\end{minipage}%
\begin{minipage}{.5\linewidth}
      \centering
        
        \scalebox{0.6}{

        \begin{tabular}{|l|c|}
        \hline \multicolumn{1}{|c|}{Proof obligations } & \provername{Alt-Ergo 2.4.1} \\ 
        \hline
        \explanation{store\_valid\_pointer\_2} & \valid{0.01} \\ 
        \hline
        \explanation{load\_alloc\_same\_2} & \valid{0.02} \\ 
        \hline
        \explanation{load\_store\_mismatch\_2} & \valid{0.02} \\ 
        \hline
        \explanation{load\_store\_overlap\_2} & \valid{0.02} \\ 
        \hline
        \explanation{load\_store\_classification} & \valid{0.01} \\ 
        \hline
        \explanation{load\_store\_characterization\_lsc\_similar} & \valid{0.01} \\ 
        \hline
        \explanation{load\_store\_characterization\_lsc\_other} & \valid{0.01} \\ 
        \hline
        \explanation{load\_store\_characterization\_lsc\_overlap} & \valid{0.01} \\ 
        \hline
        \explanation{load\_store\_characterization\_lsc\_mismatch} & \valid{0.01} \\ 
        \hline
        \explanation{store\_same\_domain} & \valid{0.02} \\ 
        \hline
        \explanation{free\_same\_domain} & \valid{0.01} \\ 
        \hline
        \explanation{free\_not\_valid\_pointer} & \valid{0.01} \\ 
        \hline \end{tabular}

        }
    \medskip
    \caption{Proof stats of REF\_GEN\_MEM}
\end{minipage} 
\end{table}

\newpage
\section{Proof statistics of module REL\_MEM and MEM\_EXTENDS}

\begin{table}[ht]
%\vspace{-15em}
\begin{minipage}{.5\linewidth}
      
    \centering
        \scalebox{0.4}{

        \begin{tabular}[ht]{|l|l|l|l|c|c|c|c|}
        \hline \multicolumn{2}{|c|}{Proof obligations } & \provername{Alt-Ergo 2.4.1} & \provername{CVC4 1.8} & \provername{Eprover 2.6} & \provername{Z3 4.8.10} \\ 
        \hline
        \explanation{valid\_pointer\_emb} & & \valid{0.05} & \noresult& \noresult& \noresult\\ 
        \hline
        \explanation{store\_unmapped\_emb}  & \explanation{store\_unmapped\_emb.0} & \noresult& \noresult& \noresult& \valid{1.27} \\ 
        \hline
        \explanation{store\_outside\_emb} & & \noresult& \noresult& \noresult& \valid{0.24} \\ 
        \hline
        \explanation{VC for store\_mapped\_emb}  & \explanation{assertion} & \valid{0.03} & \noresult& \noresult& \noresult\\ 
        \cline{2-6}
         & \explanation{assertion} & \valid{0.03} & \noresult& \noresult& \noresult\\ 
        \cline{2-6}
         & \explanation{postcondition} &  \noresult& \noresult& \noresult& \valid{14.34} \\ 
        \hline
        \explanation{alignment\_shift} & & \noresult& \noresult& \valid{0.65} & \noresult\\ 
        \hline
        \explanation{alloc\_parallel\_emb}  & \explanation{alloc\_parallel\_emb.0}  & \valid{3.44} & \noresult& \noresult& \noresult\\ 
        \hline
        \explanation{alloc\_right!\_emb} & & \noresult& \noresult& \noresult& \valid{0.07} \\ 
        \hline
        \explanation{alloc\_left\_unmapped\_emb}  & \explanation{alloc\_left\_unmapped\_emb.0} & \noresult& \noresult& \noresult& \valid{1.18} \\ 
        \hline
        \explanation{alloc\_left\_mapped\_emb}  & \explanation{alloc\_left\_mapped\_emb.0}  & \valid{1.29} & \noresult& \noresult& \noresult\\ 
        \hline
        \explanation{free\_left\_emb}  & & \noresult& \noresult& \noresult& \valid{0.67} \\ 
        \hline
        \explanation{free\_right\_emb}  & & \noresult& \noresult& \noresult& \valid{0.09} \\ 
        \hline
        \explanation{VC for free\_list\_left\_emb}  & \explanation{variant decrease}  & \valid{0.05} & \noresult& \noresult& \noresult\\ 
        \cline{2-6}
         & \explanation{precondition}  & \valid{0.02} & \noresult& \noresult& \noresult\\ 
        \cline{2-6}
         & \explanation{precondition}  & \valid{0.02} & \noresult& \noresult& \noresult\\ 
        \cline{2-6}
         & \explanation{postcondition}  & \valid{0.05} & \noresult& \noresult& \noresult\\ 
        \cline{2-6}
           &  & \noresult& \valid{0.55} & \noresult& \noresult\\ 
        \cline{2-6}
          & & \valid{0.05} & \noresult& \noresult& \noresult\\ 
        \hline
        \explanation{free\_list\_left\_emb\_original}  & & \valid{0.04} & \noresult& \noresult& \noresult\\ 
        \hline
        \explanation{VC for free\_list\_not\_valid\_block}  & \explanation{precondition}  & \valid{0.02} & \noresult& \noresult& \noresult\\ 
        \cline{2-6}
         & \explanation{postcondition}  & \valid{0.05} & \noresult& \noresult& \noresult\\ 
        \cline{2-6}
          & & \valid{0.05} & \noresult& \noresult& \noresult\\ 
        \cline{2-6}
          & & \noresult& \valid{0.47} & \noresult& \noresult\\ 
        \hline
        \explanation{free\_list\_not\_valid\_block\_original} & & \valid{0.04} & \noresult& \noresult& \noresult\\ 
        \hline
        \explanation{free\_list\_free\_parallel\_emb}  & & \valid{0.06} & \noresult& \noresult& \noresult\\ 
        \hline
        \explanation{free\_parallel\_emb} & & \valid{0.12} & \noresult& \noresult& \noresult\\ 
        \hline \end{tabular}

        }
    \medskip
    \caption{Proof stats of REL\_MEM}
\end{minipage}%
\begin{minipage}{.5\linewidth}
      \centering
        
        \scalebox{0.4}{

    \begin{tabular}[ht]{|l|l|c|c|c|}
    \hline \multicolumn{2}{|c|}{Proof obligations } & \provername{Alt-Ergo 2.4.1} & \provername{CVC4 1.8} & \provername{Z3 4.8.10} \\ 
    \hline
    \explanation{mem\_extends\_refl} & & \valid{0.22} & \noresult& \noresult\\ 
    \hline
    \explanation{mem\_extends\_trans} & & \noresult& \noresult& \valid{0.08} \\ 
    \hline
    \explanation{alloc\_extends}  & \explanation{alloc\_extends.0} & \valid{0.05} & \noresult& \noresult\\ 
    \cline{2-5}
     & \explanation{alloc\_extends.1}  &  \valid{0.05} & \noresult& \noresult\\ 
    \cline{2-5}
     &  & \noresult& \noresult& \valid{3.05} \\ 
    \hline
    \explanation{load\_extends} & & \valid{0.55} & \noresult& \noresult\\ 
    \hline
    \explanation{store\_within\_extends}  & \explanation{store\_within\_extends.0}  & \noresult& \valid{9.16} & \noresult\\ 
    \hline
    \explanation{store\_outside\_extends}  & \explanation{store\_outside\_extends.0}   & \valid{0.06} & \noresult& \noresult\\ 
    \cline{2-5}
     &   & \noresult& \noresult& \valid{2.54} \\ 
    \hline
    \explanation{free\_extends}  & \explanation{free\_extends.0}  & \valid{0.07} & \noresult& \noresult\\ 
    \cline{2-5}
     &   & \valid{27.35} & \noresult& \noresult\\ 
    \hline \end{tabular}

    }
    \medskip
    \caption{Proof stats of MEM\_EXTENDS}
\end{minipage} 
\end{table}

\section{Proof statistics of module CONCRETE\_MEM}

%Concrete_mem
\scalebox{0.5}{

\begin{tabular}{|l|c|c|c|}
\hline \multicolumn{1}{|c|}{Proof obligations } & \provername{Alt-Ergo 2.4.1} & \provername{Spass 3.7} \\ 
\hline
\explanation{update\_s} & \valid{0.01} & \noresult\\ 
\hline
\explanation{update\_o} & \valid{0.01} & \noresult\\ 
\hline
\explanation{valid\_block\_dec} & \valid{0.01} & \noresult\\ 
\hline
\explanation{zdivide\_Zmod} & \noresult& \valid{0.22} \\ 
\hline
\explanation{aligned\_dec} & \valid{0.01} & \noresult\\ 
\hline
\explanation{valid\_pointer\_dec} & \valid{0.01} & \noresult\\ 
\hline
\explanation{VC for check\_cont} & \valid{0.01} & \noresult\\ 
\hline
\explanation{VC for check\_cont\_charact\_if} & \valid{0.31} & \noresult\\ 
\hline
\explanation{VC for check\_cont\_charact\_else} & \valid{0.02} & \noresult\\ 
\hline
\explanation{check\_cont\_charact\_original} & \valid{0.01} & \noresult\\ 
\hline
\explanation{check\_cont\_exten} & \valid{0.02} & \noresult\\ 
\hline
\explanation{load\_contents\_exten} & \valid{0.05} & \noresult\\ 
\hline
\explanation{load\_contents\_1} & \valid{0.02} & \noresult\\ 
\hline
\explanation{load\_contents\_2} & \valid{0.01} & \noresult\\ 
\hline
\explanation{load\_contents\_3} & \valid{0.01} & \noresult\\ 
\hline
\explanation{load\_contents\_4} & \valid{0.02} & \noresult\\ 
\hline
\explanation{VC for set\_cont} & \valid{0.01} & \noresult \\
\hline
\explanation{VC for set\_cont\_outside} & \valid{0.02} & \noresult\\ 
\hline
\explanation{set\_cont\_outside\_original} & \valid{0.01} & \noresult\\ 
\hline
\explanation{VC for set\_cont\_inside} & \valid{0.02} & \noresult\\ 
\hline
\explanation{set\_cont\_inside\_original} & \valid{0.01} & \noresult\\ 
\hline
\explanation{store\_contents\_at} & \valid{0.01} & \noresult\\ 
\hline
\explanation{store\_contents\_cont} & \valid{0.01} & \noresult\\ 
\hline
\explanation{store\_contents\_outside} & \valid{0.02} & \noresult\\ 
\hline
\explanation{load\_store\_contents\_same} & \valid{0.04} & \noresult\\ 
\hline
\explanation{load\_store\_contents\_disjoint} & \valid{0.02} & \noresult\\ 
\hline
\explanation{load\_store\_contents\_mismatch} & \valid{0.02} & \noresult\\ 
\hline
\explanation{load\_store\_contents\_overlap} & \valid{0.02} & \noresult\\ 
\hline
\explanation{alloc\_result\_bounds\_} & \valid{0.02} & \noresult\\ 
\hline
\explanation{alloc\_bounds\_inv\_} & \valid{0.02} & \noresult\\ 
\hline
\explanation{store\_bounds\_inv\_} & \valid{0.02} & \noresult\\ 
\hline
\explanation{free\_bounds\_inv\_} & \valid{0.02} & \noresult\\ 
\hline
\explanation{fresh\_valid\_block\_exclusive\_} & \valid{0.01} & \noresult\\ 
\hline
\explanation{alloc\_fresh\_block\_} & \valid{0.02} & \noresult\\ 
\hline
\explanation{alloc\_fresh\_block\_2\_} & \valid{0.02} & \noresult\\ 
\hline
\explanation{store\_inversion} & \valid{0.02} & \noresult\\ 
\hline
\explanation{store\_fresh\_block\_} & \valid{0.02} & \noresult\\ 
\hline
\explanation{free\_fresh\_block\_} & \valid{0.02} & \noresult\\ 
\hline
\explanation{alloc\_valid\_block} & \valid{0.05} & \noresult\\ 
\hline
\explanation{alloc\_not\_valid\_block\_} & \valid{0.02} & \noresult\\ 
\hline
\explanation{load\_valid\_block\_} & \valid{0.02} & \noresult\\ 
\hline
\explanation{store\_valid\_block\_} & \valid{0.02} & \noresult\\ 
\hline
\explanation{store\_valid\_block\_inv\_} & \valid{0.02} & \noresult\\ 
\hline
\explanation{free\_valid\_block\_} & \valid{0.02} & \noresult\\ 
\hline
\explanation{store\_valid\_pointer\_inv\_} & \valid{0.03} & \noresult\\ 
\hline
\explanation{alloc\_valid\_pointer\_inv\_} & \valid{0.04} & \noresult\\ 
\hline
\explanation{free\_valid\_pointer\_inv\_} & \valid{0.03} & \noresult\\ 
\hline
\explanation{load\_alloc\_other\_} & \valid{0.05} & \noresult\\ 
\hline
\explanation{valid\_pointer\_compat\_} & \valid{0.02} & \noresult\\ 
\hline
\explanation{load\_store\_same\_} & \valid{0.07} & \noresult\\ 
\hline
\explanation{load\_store\_disjoint\_} & \valid{0.24} & \noresult\\ 
\hline
\explanation{load\_free\_other\_} & \valid{0.02} & \noresult\\ 
\hline
\explanation{load\_alloc\_same\_} & \valid{0.05} & \noresult\\ 
\hline
\explanation{load\_store\_mismatch\_} & \valid{0.04} & \noresult\\ 
\hline
\explanation{load\_store\_overlap\_} & \valid{0.05} & \noresult\\ 
\hline
\explanation{same\_domain\_same\_nextblock} & \valid{0.05} & \noresult\\ 
\hline
\explanation{alloc\_same\_domain\_} & \valid{0.11} & \noresult\\ 
\hline
\explanation{valid\_block\_free\_} & \valid{0.02} & \noresult\\ 
\hline
\explanation{valid\_pointer\_store\_} & \valid{0.02} & \noresult\\ 
\hline
\explanation{store\_valid\_pointer\_} & \valid{0.02} & \noresult\\ 
\hline
\explanation{valid\_pointer\_load\_} & \valid{0.02} & \noresult\\ 
\hline
\explanation{load\_valid\_pointer\_} & \valid{0.02} & \noresult\\ 
\hline
\explanation{free\_not\_valid\_block\_} & \valid{0.03} & \noresult\\ 
\hline
\explanation{free\_same\_bounds\_} & \valid{0.02} & \noresult\\ 
\hline \end{tabular}

}

\section{Proof statistics of module MEM\_LESSDEF}

\scalebox{0.5}{

\begin{tabular}{|l|l|c|c|c|}
\hline \multicolumn{2}{|c|}{Proof obligations } & \provername{Alt-Ergo 2.4.1} & \provername{CVC4 1.8} & \provername{Z3 4.8.10} \\ 
\hline
\explanation{mem\_lessdef\_refl} & & \valid{0.35} & \noresult& \noresult\\ 
\hline
\explanation{mem\_lessdef\_trans}  & \explanation{mem\_lessdef\_trans.0} & \noresult& \noresult& \valid{0.53} \\ 
\hline
\explanation{VC for alloc\_lessdef}  & \explanation{assertion} &  \valid{0.10} & \noresult& \noresult\\ 
\cline{2-5}
 & \explanation{assertion} & \noresult& \noresult& \valid{0.08} \\ 
\cline{2-5}
 & \explanation{postcondition}  &  \valid{0.08} & \noresult& \noresult\\ 
\cline{2-5}
 &  &  \valid{0.03} & \noresult& \noresult\\ 
\cline{2-5}
 &  &   \noresult& \valid{11.87} & \noresult\\ 
\hline
\explanation{load\_lessdef} & & \valid{0.71} & \noresult& \noresult\\ 
\hline
\explanation{VC for store\_lessdef}  & \explanation{assertion}  & \noresult& \noresult& \valid{0.18} \\ 
\cline{2-5}
 & \explanation{assertion} & \valid{0.07} & \noresult& \noresult\\ 
\cline{2-5}
 & \explanation{assertion} & \valid{0.09} & \noresult& \noresult\\ 
\cline{2-5}
 & \explanation{assertion} & \valid{0.06} & \noresult& \noresult\\ 
\cline{2-5}
 & \explanation{assertion} & \noresult& \noresult& \valid{0.13} \\ 
\cline{2-5}
 & \explanation{assertion} & \valid{0.02} & \noresult& \noresult\\ 
\cline{2-5}
 & \explanation{assertion} & \valid{0.06} & \noresult& \noresult\\ 
\cline{2-5}
 & \explanation{assertion} & \valid{0.06} & \noresult& \noresult\\ 
\cline{2-5}
 & \explanation{assertion} & \valid{0.02} & \noresult& \noresult\\ 
\cline{2-5}
 & \explanation{assertion} & \valid{0.06} & \noresult& \noresult\\ 
\cline{2-5}
 & \explanation{postcondition}  & \valid{0.07} & \noresult& \noresult\\ 
\cline{2-5}
 &  &  \valid{1.34} & \noresult& \noresult\\ 
\hline
\explanation{store\_lessdef\_original} & & \valid{0.08} & \noresult& \noresult\\ 
\hline
\explanation{free\_lessdef}  & \explanation{free\_lessdef.0}  & \valid{0.08} & \noresult& \noresult\\ 
\cline{2-5}
 &  &  \noresult& \valid{0.45} & \noresult\\ 
\hline \end{tabular}

}

\section{Proof statistics of module MEM\_INJECT}

%MEM_INJECT
\scalebox{0.4}{

\begin{tabular}{|l|l|c|c|c|c|}
\hline \multicolumn{2}{|c|}{Proof obligations } & \provername{Alt-Ergo 2.4.1} & \provername{CVC4 1.8} & \provername{Z3 4.8.10} & \provername{Z3 4.8.5} \\ 
\hline
\explanation{load\_inject} & & \noresult& \noresult& \valid{0.54} & \noresult \\ 
\hline
\explanation{VC for store\_mapped\_inject}  & \explanation{assertion} & \noresult& \noresult& \valid{2.16} & \noresult \\ 
\cline{2-6}
 & \explanation{postcondition}  & \valid{1.00} & \noresult& \noresult& \noresult\\ 
\hline
\explanation{store\_unmapped\_inject} & & \valid{0.08} & \noresult& \noresult& \noresult\\ 
\hline
\explanation{VC for loadv\_inject} & & \noresult& \noresult& \valid{0.31} & \noresult\\ 
\hline
\explanation{VC for storev\_inject} & & \noresult& \valid{0.30} & \noresult& \noresult\\ 
\hline
\explanation{embedding\_no\_overlap\_free} & & \valid{0.06} & \noresult& \noresult& \noresult\\ 
\hline
\explanation{VC for embedding\_no\_overlap\_free\_list}  & \explanation{precondition} & \valid{0.04} & \noresult& \noresult& \noresult\\ 
\cline{2-6}
 & \explanation{precondition} &  \valid{0.04} & \noresult& \noresult& \noresult\\ 
\cline{2-6}
 & \explanation{postcondition}  &  \valid{0.05} & \noresult& \noresult& \noresult\\ 
\cline{2-6}
 &  &   \noresult& \valid{0.41} & \noresult& \noresult\\ 
\cline{2-6}
 &  &  \valid{0.06} & \noresult& \noresult& \noresult\\ 
\hline
\explanation{VC for free\_list\_fresh\_block}  & \explanation{precondition} & \valid{0.04} & \noresult& \noresult& \noresult\\ 
\cline{2-6}
 & \explanation{postcondition}  &  \valid{0.05} & \noresult& \noresult& \noresult\\ 
\cline{2-6}
 &  &  \noresult& \valid{0.46} & \noresult& \noresult\\ 
\cline{2-6}
 &  & \valid{0.06} & \noresult& \noresult& \noresult\\ 
\cline{2-6}
 &  &  \valid{0.06} & \noresult& \noresult& \noresult\\ 
\cline{2-6}
 &  &  \noresult& \valid{0.64} & \noresult& \noresult\\ 
\cline{2-6}
 &  &  \valid{0.05} & \noresult& \noresult& \noresult\\ 
\hline
\explanation{free\_inject} & & \valid{0.07} & \noresult& \noresult& \noresult\\ 
\hline
\explanation{extend\_embedding\_incr} & & \valid{0.04} & \noresult& \noresult& \noresult\\ 
\hline
\explanation{alloc\_right\_inject} & & \valid{0.06} & \noresult& \noresult& \noresult\\ 
\hline
\explanation{alloc\_left\_unmapped\_inject}  & \explanation{alloc\_left\_unmapped\_inject.0}  & \noresult& \valid{0.29} & \noresult& \noresult\\ 
\cline{2-6}
 &   & \valid{0.06} & \noresult& \noresult& \noresult\\ 
\cline{2-6}
 &   & \valid{0.06} & \noresult& \noresult& \noresult\\ 
\cline{2-6}
 &   & \valid{0.09} & \noresult& \noresult& \noresult\\ 
\cline{2-6}
 & \explanation{alloc\_left\_unmapped\_inject.1} & \valid{0.10} & \noresult& \noresult& \noresult\\ 
\hline
\explanation{alloc\_left\_mapped\_inject}  & \explanation{alloc\_left\_mapped\_inject.0}   & \valid{4.01} & \noresult& \noresult& \noresult\\ 
\cline{2-6}
 &  &  \valid{0.10} & \noresult& \noresult& \noresult\\ 
\cline{2-6}
 &  &  \valid{0.10} & \noresult& \noresult& \noresult\\ 
\cline{2-6}
 &  &  \valid{0.32} & \noresult& \noresult& \noresult\\ 
\cline{2-6}
 & \explanation{alloc\_left\_mapped\_inject.1} & \valid{0.13} & \noresult& \noresult& \noresult\\ 
\hline
\explanation{alloc\_list\_unfold} & & \valid{0.23} & \noresult& \noresult& \noresult\\ 
\hline
\explanation{VC for alloc\_list\_left\_inject}  & \explanation{assertion} & \valid{0.13} & \noresult& \noresult& \noresult\\ 
\cline{2-6}
 & \explanation{assertion} & \noresult& \noresult& \valid{0.14} & \noresult\\ 
\cline{2-6}
 & \explanation{assertion} & \noresult& \noresult& \valid{0.13} & \noresult\\ 
\cline{2-6}
 & \explanation{assertion}  & \valid{0.08} & \noresult& \noresult& \noresult\\ 
\cline{2-6}
 &  & \noresult& \noresult& \valid{0.69} & \noresult\\ 
\cline{2-6}
 &  &  \valid{0.11} & \noresult& \noresult& \noresult\\ 
\cline{2-6}
 & \explanation{assertion} & \valid{0.33} & \noresult& \noresult& \noresult\\ 
\cline{2-6}
 & \explanation{assertion} & \valid{0.18} & \noresult& \noresult& \noresult\\ 
\cline{2-6}
 & \explanation{assertion} & \valid{0.14} & \noresult& \noresult& \noresult\\ 
\cline{2-6}
 & \explanation{assertion}  & \valid{0.09} & \noresult& \noresult& \noresult\\ 
\cline{2-6}
 &  &  \valid{0.09} & \noresult& \noresult& \noresult\\ 
\cline{2-6}
 &  & \noresult& \noresult& \valid{0.17} & \noresult\\ 
\cline{2-6}
 & \explanation{assertion} & \valid{0.14} & \noresult& \noresult& \noresult\\ 
\cline{2-6}
 & \explanation{precondition} & \valid{0.05} & \noresult& \noresult& \noresult\\ 
\cline{2-6}
 & \explanation{precondition} & \valid{0.06} & \noresult& \noresult& \noresult\\ 
\cline{2-6}
 & \explanation{precondition} & \valid{0.06} & \noresult& \noresult& \noresult\\ 
\cline{2-6}
 & \explanation{precondition} & \valid{0.06} & \noresult& \noresult& \noresult\\ 
\cline{2-6}
 & \explanation{precondition} & \valid{0.19} & \noresult& \noresult& \noresult\\ 
\cline{2-6}
 & \explanation{postcondition}  & \noresult& \noresult& \noresult& \valid{0.05} \\ 
\cline{2-6}
 &  &  \noresult& \noresult& \noresult& \valid{0.05} \\ 
\cline{2-6}
 &  &  \noresult& \noresult& \noresult& \valid{0.05} \\ 
\cline{2-6}
 &  &  \noresult& \noresult& \noresult& \valid{0.04} \\ 
\cline{2-6}
 &  & \noresult& \valid{0.47} & \noresult& \noresult\\ 
\cline{2-6}
 &  & \noresult& \noresult& \noresult& \valid{0.04} \\ 
\cline{2-6}
 &  &  \noresult& \noresult& \noresult& \valid{0.03} \\ 
\cline{2-6}
 &  & \noresult& \noresult& \noresult& \valid{0.04} \\ 
\cline{2-6}
 &  & \noresult& \noresult& \noresult& \valid{0.08} \\ 
\cline{2-6}
 &  & \noresult& \noresult& \noresult& \valid{0.20} \\ 
\cline{2-6}
 &  & \noresult& \noresult& \noresult& \valid{0.02} \\ 
\hline
\explanation{VC for alloc\_list\_left\_inject\_original} & & \noresult& \valid{0.18} & \noresult& \noresult\\ 
\hline
\explanation{VC for alloc\_list\_alloc\_inject}  & \explanation{assertion} & \valid{0.15} & \noresult& \noresult& \noresult\\ 
\cline{2-6}
 & \explanation{assertion} & \valid{0.15} & \noresult& \noresult& \noresult\\ 
\cline{2-6}
 & \explanation{assertion} & \valid{0.16} & \noresult& \noresult& \noresult\\ 
\cline{2-6}
 & \explanation{assertion} & \valid{0.15} & \noresult& \noresult& \noresult\\ 
\cline{2-6}
 & \explanation{assertion}  &  \noresult& \valid{3.32} & \noresult& \noresult\\ 
\cline{2-6}
 & \explanation{postcondition}  &  \noresult& \valid{2.82} & \noresult& \noresult\\ 
\hline \end{tabular}

}
